# Supplementary material for: DART2: a robust multiple testing method to smartly leverage helpful or misleading ancillary information
Source: arXiv:2409.03618 source file (2024-09-05)
Supplement: Supplementary file 1 [file supp.tex]

% ======================================================================
% Supplementary Materials
% ======================================================================

%% HACKS %%

% Reset all the counts.
\setcounter{section}{0}
\setcounter{subsection}{0}
\setcounter{equation}{0}
\setcounter{figure}{0}
\setcounter{table}{0}
\setcounter{page}{1}

% For section headers starting with S

% Hack for making SOM Equations Conform to Science Format
%
% e.g. (S1), (S2), etc
% Requires AMS

%\makeatletter %% With ams
%\def\tagform@#1{\maketag@@@{(S\ignorespaces#1\unskip\@@italiccorr)}}
%\makeatother
 
% Hack for making figures Say \figurename S\thefigure, e.g. Figure S1:
%\makeatletter
%\makeatletter \renewcommand{\fnum@figure}
%{\figurename~S\thefigure}
%\makeatother
 
% use bibnumfmt to change style at the end of the document

% citenumfont command adds S to all numbers

%END HACKS

%\makeatletter %% HAVE TO ADD SOMETHING HERE TO MAKE IT SAY "APPENDIX"
% \renewcommand{\@seccntformat}[1]{APPENDIX~{\csname
% the#1\endcsname}.\hspace*{1em}} \makeatother
\newpage
\begin{center}
{\large
\textbf{Supplementary Materials}
}
\end{center}

%%% Local Variables:
%%% mode: latex
%%% TeX-master: "../manu"
%%% End:
